# Supplementary material for: Bandit Guided Submodular Curriculum for Adaptive Subset Selection
Source: arXiv:2511.22944 source file (2025-11-28)
Supplement: Supplementary file 1 [file technicalAppendix.tex]

\newpage
\onecolumn
\allowdisplaybreaks
\par\noindent\rule{\textwidth}{1pt}
\begin{center}
\large\textbf{Reproducibility Checklist: 
\papertitle}
\end{center}
\par\noindent\rule{\textwidth}{0.4pt}

\section{Reproducibility Checklist}\label{ref:Checklist}
\begin{itemize}
    \item Includes a conceptual outline and/or pseudocode description of AI methods introduced (\textbf{yes})
 \item Clearly delineates statements that are opinions, hypothesis, and speculation from objective facts and results (\textbf{yes})
 \item Provides well marked pedagogical references for less-familiare readers to gain background necessary to replicate the paper (\textbf{yes})

\item Does this paper make theoretical contributions? \textbf{yes}

\textbf{If yes, please complete the list below.}

\item All assumptions and restrictions are stated clearly and formally. \textbf{yes}
\item All novel claims are stated formally (e.g., in theorem statements). \textbf{yes}
\item Proofs of all novel claims are included. \textbf{yes}
\item Proof sketches or intuitions are given for complex and/or novel results. \textbf{yes}
\item Appropriate citations to theoretical tools used are given. (\textbf{yes})
\item All theoretical claims are demonstrated empirically to hold. (\textbf{partial})
\item All experimental code used to eliminate or disprove claims is included. (\textbf{yes})
\item Does this paper rely on one or more datasets? (\textbf{yes})

If yes, please complete the list below.

\item A motivation is given for why the experiments are conducted on the selected datasets (\textbf{partial})
\item All novel datasets introduced in this paper are included in a data appendix. (\textbf{NA})
\item All novel datasets introduced in this paper will be made publicly available upon publication of the paper with a license that allows free usage for research purposes. (\textbf{NA})
\item All datasets drawn from the existing literature (potentially including authors’ own previously published work) are accompanied by appropriate citations. (yes/no/NA)
\item All datasets drawn from the existing literature (potentially including authors’ own previously published work) are publicly available. (\textbf{yes})
\item All datasets that are not publicly available are described in detail, with explanation why publicly available alternatives are not scientifically satisfying. (\textbf{NA})
\item Does this paper include computational experiments? (\textbf{no})

\textbf{If yes, please complete the list below.
}
\item Any code required for pre-processing data is included in the appendix. (\textbf{no}).
\item All source code required for conducting and analyzing the experiments is included in a code appendix. (\textbf{yes})
\item All source code required for conducting and analyzing the experiments will be made publicly available upon publication of the paper with a license that allows free usage for research purposes. (\textbf{yes})
\item All source code implementing new methods have comments detailing the implementation, with references to the paper where each step comes from (\textbf{partial})
\item If an algorithm depends on randomness, then the method used for setting seeds is described in a way sufficient to allow replication of results. (\textbf{yes})
\item This paper specifies the computing infrastructure used for running experiments (hardware and software), including GPU/CPU models; amount of memory; operating system; names and versions of relevant software libraries and frameworks. (\textbf{yes})
\item This paper formally describes evaluation metrics used and explains the motivation for choosing these metrics. (\textbf{yes})
\item This paper states the number of algorithm runs used to compute each reported result. (\textbf{yes})
\item Analysis of experiments goes beyond single-dimensional summaries of performance (e.g., average; median) to include measures of variation, confidence, or other distributional information. \textbf{no}
\item The significance of any improvement or decrease in performance is judged using appropriate statistical tests (e.g., Wilcoxon signed-rank). (\textbf{partial})
\item This paper lists all final (hyper-)parameters used for each model/algorithm in the paper’s experiments. \textbf{yes}
\item This paper states the number and range of values tried per (hyper-) parameter during development of the paper, along with the criterion used for selecting the final parameter setting. \textbf{yes}

\end{itemize}
